# Supplementary material for: A New Defense Against Adversarial Images: Turning a Weakness into a Strength
Source: arXiv:1910.07629 source file (2019-12-04)
Supplement: Supplementary file 1 [file appendix.tex]

%!TEX root=main.tex

\begin{table}[t!]
  \centering
  \begin{tabular}{llllllll}
    \toprule
    \multirow{2}{*}{Detector}&\multirow{2}{*}{FPR}&\multicolumn{2}{c}{LR=0.01}  &  \multicolumn{2}{c}{LR=0.03} &  \multicolumn{2}{c}{LR=0.1}       \\
    \cmidrule(l){3-4}
    \cmidrule(l){5-6}
    \cmidrule(l){7-8}
        & & PGD & CW & PGD & CW & PGD & CW \\
    \midrule
    C1 &0.2& 0.858& 0.803& 0.712& 0.483&0.628&0.368\\
    C2a &0.2&0.173&0.449&0.411&0.585&0.424&0.543\\
    C2b &0.2&0.004&0.346&0.013&0.225&0.003&0.067\\
    Combined &0.2&0.762&0.788&0.546&0.527&0.468&0.479\\
    \midrule
    C1 &0.1& 0.648& 0.688& 0.360& 0.290&0.258&0.142\\
    C2a &0.1&0.043&0.231&0.157&0.322&0.180&0.321\\
    C2b &0.1&0.001&0.255&0.006&0.114&0.003&0.056\\
    Combined &0.1&0.762&0.788&0.546&0.527&0.468&0.479\\
    \midrule
    Feature Squeezing & -&-&-&0.0&0.054&-&-\\
    \bottomrule
  \end{tabular}
  \caption{Imagenet Whitebox: Inception}
  \label{tab:rates_inception}
\end{table}

\eat{
\begin{table}[t]
\begin{threeparttable}
\caption{Transformation ensemble performance in different neighborhood with VGG19 on Greybox Attack 1 noise}
\label{sample-table}
\vskip 0.15in
\begin{center}
\begin{small}
\begin{sc}
\begin{tabular}{lccccr}
\toprule
attack & detection   &     2\% &    5\% &    10\% &    20\% \\
\midrule
 \multirow{6}{2em}{AUG-PGD}&baseline &na& 82.38 & 88.99 & 94.39 \\
 &noise-free& 65.07&87.21&-&96.89\\
 &$\epsilon$=0.01 & 70.56 & 85.78 & 89.11 & 96.78 \\
 &$\epsilon$=0.03 & 73.33 & 84.89 & 90.44 & 96.33 \\
 &$\epsilon$=0.05 & 73.33 & 85.33 & 90.56 & 96.56 \\
 &$\epsilon$=0.07 & 75.44 & 86.11 & 92.33 & 96.67 \\
 &$\epsilon$=0.09 & 76.00 & 86.78 & 92.78 & 97.56 \\
\midrule
 \multirow{6}{2em}{Alt-PGD}&baseline &na& 72.14 & 77.96 & 87.88 \\
 &noise-free&43.88&74.39&-&93.43\\
 &$\epsilon$=0.01 & 50.17 & 73.30 & 77.31 & 92.66 \\
 &$\epsilon$=0.03 & 53.39 & 74.64 & 79.87 & 92.55 \\
 &$\epsilon$=0.05 & 57.17 & 74.53 & 82.65 & 92.77 \\
 &$\epsilon$=0.07 & 57.84 & 74.19 & 82.87 & 92.88 \\
 &$\epsilon$=0.09 & 59.62 & 76.75 & 84.87 & 92.66 \\
 \midrule
 \multirow{6}{2em}{FGSM}&baseline &na& 38.20 & 57.54 & 74.57 \\
 &noise-free&26.63&46.33&-&77.17\\
 &$\epsilon$=0.01 & 30.12 & 42.06 & 51.83 & 73.00 \\
 &$\epsilon$=0.03 & 31.34 & 45.05 & 54.00 & 74.08 \\
 &$\epsilon$=0.05 & 31.21 & 43.83 & 55.50 & 74.90 \\
 &$\epsilon$=0.07 & 32.56 & 45.73 & 57.80 & 74.90 \\
 &$\epsilon$=0.09 & 32.84 & 45.05 & 59.16 & 78.56 \\
 \midrule
 \multirow{6}{2em}{T-FGSM}&baseline &na& 40.85 & 63.00 & 81.56 \\
 &noise-free&32.72&55.9&-&82.36\\
 &$\epsilon$=0.01 & 38.07 & 51.56 & 59.94 & 79.83 \\
 &$\epsilon$=0.03 & 38.78 & 51.56 & 63.92 & 81.82 \\
 &$\epsilon$=0.05 & 38.49 & 53.84 & 64.91 & 80.97 \\
 &$\epsilon$=0.07 & 39.35 & 54.12 & 65.48 & 82.39 \\
 &$\epsilon$=0.09 & 39.91 & 53.84 & 66.19 & 82.53 \\
 \midrule
 \multirow{6}{2em}{I-FGSM}&baseline &na& 41.49 & 51.89 & 65.55 \\
 &noise-free&24.43&45.48&-&79.75\\
 &$\epsilon$=0.01 & 26.67 & 43.16 & 50.96 & 76.84 \\
 &$\epsilon$=0.03 & 29.38 & 44.75 & 53.56 & 77.18 \\
 &$\epsilon$=0.05 & 29.72 & 42.60 & 54.35 & 77.51 \\
 &$\epsilon$=0.07 & 31.53 & 44.29 & 59.32 & 78.19 \\
 &$\epsilon$=0.09 & 30.73 & 44.41 & 58.87 & 79.21 \\

\bottomrule
\end{tabular}
\end{sc}
\end{small}
\end{center}
\vskip -0.1in
\begin{tablenotes}
      \small
      \item The five cells 
    \end{tablenotes}
  \end{threeparttable}
\end{table}

\begin{table}[t]
\begin{threeparttable}
\caption{Transformation ensemble performance in different neighborhood with VGG19 on Greybox Attack 3 noise}
\label{sample-table}
\vskip 0.15in
\begin{center}
\begin{small}
\begin{sc}
\begin{tabular}{lccccr}
\toprule
attack & detection   &     2\% &    5\% &    10\% &    20\% \\
\midrule
 \multirow{6}{2em}{AUG-PGD}&baseline &na& 82.38 & 88.99 & 94.39 \\
&$\epsilon$=0.01 & 67.33 & 84.78 & 91.00 & 97.33 \\
 &$\epsilon$=0.03 & 70.44 & 83.33 & 89.89 & 96.56 \\
 &$\epsilon$=0.05 & 71.56 & 84.89 & 90.44 & 96.22 \\
 &$\epsilon$=0.07 & 73.67 & 84.33 & 92.00 & 96.56 \\
 &$\epsilon$=0.09 & 75.33 & 85.89 & 89.33 & 94.67 \\
\midrule
 \multirow{6}{2em}{Alt-PGD}&baseline &na& 72.14 & 77.96 & 87.88 \\
&$\epsilon$=0.01 & 49.61 & 71.86 & 78.87 & 93.33 \\
 &$\epsilon$=0.03 & 53.06 & 71.86 & 80.20 & 92.66 \\
 &$\epsilon$=0.05 & 54.39 & 72.41 & 82.54 & 93.21 \\
 &$\epsilon$=0.07 & 56.28 & 73.64 & 84.76 & 92.77 \\
 &$\epsilon$=0.09 & 58.51 & 76.64 & 81.65 & 90.88 \\
 \midrule
 \multirow{6}{2em}{FGSM}&baseline &na& 38.20 & 57.54 & 74.57 \\
&$\epsilon$=0.01 & 28.63 & 41.38 & 55.63 & 75.03 \\
 &$\epsilon$=0.03 & 29.58 & 41.38 & 54.00 & 73.95 \\
 &$\epsilon$=0.05 & 30.53 & 43.28 & 54.95 & 72.18 \\
 &$\epsilon$=0.07 & 30.80 & 43.69 & 57.12 & 73.81 \\
 &$\epsilon$=0.09 & 29.17 & 43.42 & 52.65 & 65.13 \\
 \midrule
 \multirow{6}{2em}{T-FGSM}&baseline &na& 40.85 & 63.00 & 81.56 \\
&$\epsilon$=0.01 & 35.94 & 50.00 & 65.48 & 80.97 \\
 &$\epsilon$=0.03 & 37.07 & 49.57 & 63.07 & 78.98 \\
 &$\epsilon$=0.05 & 37.50 & 50.71 & 62.78 & 78.12 \\
 &$\epsilon$=0.07 & 36.93 & 51.42 & 64.91 & 81.11 \\
 &$\epsilon$=0.09 & 36.93 & 54.69 & 62.07 & 73.72 \\
 \midrule
 \multirow{6}{2em}{I-FGSM}&baseline &na& 41.49 & 51.89 & 65.55 \\
&$\epsilon$=0.01 & 25.20 & 40.00 & 53.45 & 79.55 \\
 &$\epsilon$=0.03 & 27.01 & 41.36 & 51.07 & 75.03 \\
 &$\epsilon$=0.05 & 28.02 & 43.50 & 53.79 & 73.90 \\
 &$\epsilon$=0.07 & 27.01 & 43.62 & 55.82 & 74.92 \\
 &$\epsilon$=0.09 & 28.59 & 43.73 & 51.07 & 66.10 \\

\bottomrule
\end{tabular}
\end{sc}
\end{small}
\end{center}
\vskip -0.1in
\begin{tablenotes}
      \small
      \item The five cells 
    \end{tablenotes}
  \end{threeparttable}
\end{table}

\begin{table}[t]
\begin{threeparttable}
\caption{Transformation ensemble performance in different neighborhood with VGG19 on Greybox Attack 7 noise}
\label{sample-table}
\vskip 0.15in
\begin{center}
\begin{small}
\begin{sc}
\begin{tabular}{lccccr}
\toprule
attack & detection   &     2\% &    5\% &    10\% &    20\% \\
\midrule
 \multirow{6}{2em}{AUG-PGD}&baseline &na& 82.38 & 88.99 & 94.39 \\
&$\epsilon$=0.01 & 74.30 & 85.87 & 92.21 & 96.77 \\
 &$\epsilon$=0.03 & 72.67 & 84.89 & 90.56 & 96.44 \\
 &$\epsilon$=0.05 & 75.22 & 85.78 & 91.00 & 96.11 \\
 &$\epsilon$=0.07 & 75.67 & 86.56 & 91.56 & 96.11 \\
 &$\epsilon$=0.09 & 74.33 & 87.00 & 92.00 & 95.67 \\
\midrule
 \multirow{6}{2em}{Alt-PGD}&baseline &na& 72.14 & 77.96 & 87.88 \\
&$\epsilon$=0.01 & 56.24 & 74.05 & 80.85 & 93.21 \\
 &$\epsilon$=0.03 & 55.51 & 73.41 & 80.98 & 93.21 \\
 &$\epsilon$=0.05 & 57.40 & 75.75 & 81.09 & 91.55 \\
 &$\epsilon$=0.07 & 61.51 & 76.97 & 84.98 & 92.32 \\
 &$\epsilon$=0.09 & 58.84 & 75.31 & 83.87 & 91.99 \\
 \midrule
 \multirow{6}{2em}{FGSM}&baseline &na& 38.20 & 57.54 & 74.57 \\
&$\epsilon$=0.01 & 33.02 & 44.02 & 60.05 & 74.32 \\
 &$\epsilon$=0.03 & 30.94 & 44.10 & 55.63 & 74.76 \\
 &$\epsilon$=0.05 & 31.89 & 44.37 & 54.00 & 72.73 \\
 &$\epsilon$=0.07 & 31.89 & 45.59 & 56.17 & 72.46 \\
 &$\epsilon$=0.09 & 28.49 & 43.96 & 55.90 & 70.01 \\
 \midrule
 \multirow{6}{2em}{T-FGSM}&baseline &na& 40.85 & 63.00 & 81.56 \\
&$\epsilon$=0.01 & 38.69 & 53.06 & 67.14 & 81.08 \\
 &$\epsilon$=0.03 & 38.64 & 52.41 & 65.91 & 80.40 \\
 &$\epsilon$=0.05 & 39.35 & 55.68 & 63.78 & 78.41 \\
 &$\epsilon$=0.07 & 39.35 & 56.68 & 65.48 & 80.82 \\
 &$\epsilon$=0.09 & 36.36 & 52.27 & 63.92 & 78.41 \\
 \midrule
 \multirow{6}{2em}{I-FGSM}&baseline &na& 41.49 & 51.89 & 65.55 \\
&$\epsilon$=0.01 & 29.75 & 43.33 & 56.00 & 78.05 \\
 &$\epsilon$=0.03 & 27.57 & 42.82 & 53.56 & 76.27 \\
 &$\epsilon$=0.05 & 29.94 & 44.52 & 53.11 & 72.32 \\
 &$\epsilon$=0.07 & 31.64 & 45.08 & 54.92 & 73.22 \\
 &$\epsilon$=0.09 & 27.80 & 44.18 & 54.92 & 69.15 \\

\bottomrule
\end{tabular}
\end{sc}
\end{small}
\end{center}
\vskip -0.1in
\begin{tablenotes}
      \small
      \item The five cells 
    \end{tablenotes}
  \end{threeparttable}
\end{table}

\begin{table}[t]
\begin{threeparttable}
\caption{Transformation ensemble performance in different neighborhood with VGG19 on Blackbox Attack 1 noise}
\label{sample-table}
\vskip 0.15in
\begin{center}
\begin{small}
\begin{sc}
\begin{tabular}{lccccr}
\toprule
attack&detection   &     2\% &    5\% &    10\% &    20\% \\
\midrule
\multirow{6}{2em}{AUG-PGD}&baseline& na&60.61 & 85.19  & 95.29 \\
&noise-free & 44.61 & 74.35 & - & 93.31\\
&$\epsilon$=0.01 & 50.74 & 73.33 & 81.85 & 93.70 \\
 &$\epsilon$=0.03 & 54.44 & 71.85 & 81.85 & 92.22 \\
 &$\epsilon$=0.05 & 52.96 & 72.22 & 81.85 & 92.96 \\
 &$\epsilon$=0.07 & 54.44 & 71.85 & 83.33 & 92.59 \\
 &$\epsilon$=0.09 & 52.22 & 72.96 & 83.33 & 94.07 \\
\midrule
\multirow{6}{2em}{Alt-PGD}&baseline&na& 64.58 & 83.07 & 93.73 \\
&noise-free&50.53&75.62&-&93.29\\
 &$\epsilon$=0.01 & 56.69 & 73.59 & 79.58 & 91.90 \\
 &$\epsilon$=0.03 & 56.69 & 76.41 & 83.10 & 92.96 \\
 &$\epsilon$=0.05 & 60.21 & 75.35 & 83.45 & 90.14 \\
 &$\epsilon$=0.07 & 58.10 & 73.94 & 84.15 & 92.61 \\
 &$\epsilon$=0.09 & 57.04 & 74.30 & 85.21 & 94.01 \\
\midrule
\multirow{6}{2em}{fgsm}&baseline&na& 59.00 & 80.33  & 91.84 \\
& noise-free &49.12&77.39&-&92.58\\
&$\epsilon$=0.01 & 54.48 & 67.92 & 76.89 & 90.09 \\
 &$\epsilon$=0.03 & 54.72 & 70.05 & 78.07 & 90.09 \\
 &$\epsilon$=0.05 & 55.66 & 69.10 & 78.54 & 91.75 \\
 &$\epsilon$=0.07 & 54.48 & 70.05 & 79.95 & 91.51 \\
 &$\epsilon$=0.09 & 54.95 & 69.10 & 80.66 & 92.69 \\
\midrule
\multirow{6}{2em}{t-fgsm}&baseline&na& 59.71 & 83.47 & 95.04 \\
& noise-free & 50.12&77.03&-&93.01\\
 &$\epsilon$=0.01 & 56.25 & 71.99 & 81.02 & 91.44 \\
 &$\epsilon$=0.03 & 56.94 & 73.15 & 84.03 & 92.36 \\
 &$\epsilon$=0.05 & 57.87 & 72.92 & 83.80 & 93.75 \\
 &$\epsilon$=0.07 & 57.87 & 73.15 & 84.26 & 91.90 \\
 &$\epsilon$=0.09 & 57.18 & 74.31 & 82.64 & 92.82 \\
\midrule
\multirow{6}{2em}{i-fgsm}&baseline&na& 58.42 & 76.37 & 88.83 \\
& noise-free&43.42&69.14&-&90.74\\
 &$\epsilon$=0.01 & 47.84 & 66.12 & 75.98 & 89.53 \\
 &$\epsilon$=0.03 & 47.43 & 65.09 & 75.98 & 89.12 \\
 &$\epsilon$=0.05 & 49.28 & 67.35 & 76.39 & 90.76 \\
 &$\epsilon$=0.07 & 48.46 & 65.30 & 78.03 & 91.38 \\
 &$\epsilon$=0.09 & 49.28 & 66.32 & 79.06 & 90.97 \\

\bottomrule
\end{tabular}
\end{sc}
\end{small}
\end{center}
\vskip -0.1in
\begin{tablenotes}
      \small
      \item The five cells 
    \end{tablenotes}
  \end{threeparttable}
\end{table}

\begin{table}[t]
\begin{threeparttable}
\caption{Transformation ensemble performance in different neighborhood with VGG19 on Blackbox Attack 3 noise}
\label{sample-table}
\vskip 0.15in
\begin{center}
\begin{small}
\begin{sc}
\begin{tabular}{lccccr}
\toprule
attack&detection   &     2\% &    5\% &    10\% &    20\% \\
\midrule
\multirow{6}{2em}{AUG-PGD}&baseline& na&60.61 & 85.19  & 95.29 \\
&$\epsilon$=0.01 & 48.89 & 71.11 & 83.70 & 94.07 \\
 &$\epsilon$=0.03 & 52.59 & 71.48 & 80.00 & 91.48 \\
 &$\epsilon$=0.05 & 49.63 & 69.63 & 81.11 & 90.74 \\
 &$\epsilon$=0.07 & 48.52 & 70.37 & 82.96 & 92.22 \\
 &$\epsilon$=0.09 & 50.00 & 70.00 & 79.26 & 89.63 \\
\midrule
\multirow{6}{2em}{Alt-PGD}&baseline&na& 64.58 & 83.07 & 93.73 \\
 &$\epsilon$=0.01 & 54.58 & 69.01 & 82.75 & 91.90 \\
 &$\epsilon$=0.03 & 57.39 & 73.59 & 83.10 & 91.55 \\
 &$\epsilon$=0.05 & 57.04 & 73.24 & 82.75 & 92.25 \\
 &$\epsilon$=0.07 & 58.45 & 70.42 & 84.15 & 92.61 \\
 &$\epsilon$=0.09 & 55.63 & 72.54 & 78.87 & 86.62 \\
\midrule
\multirow{6}{2em}{fgsm}&baseline&na& 59.00 & 80.33  & 91.84 \\
&$\epsilon$=0.01 & 50.47 & 68.16 & 79.72 & 90.57 \\
 &$\epsilon$=0.03 & 50.00 & 66.27 & 76.89 & 89.86 \\
 &$\epsilon$=0.05 & 50.24 & 68.16 & 78.77 & 90.09 \\
 &$\epsilon$=0.07 & 52.59 & 69.10 & 79.95 & 90.09 \\
 &$\epsilon$=0.09 & 50.47 & 68.40 & 74.29 & 85.85 \\
\midrule
\multirow{6}{2em}{t-fgsm}&baseline&na& 59.71 & 83.47 & 95.04 \\
 &$\epsilon$=0.01 & 50.93 & 70.60 & 84.26 & 93.06 \\
 &$\epsilon$=0.03 & 53.24 & 69.44 & 81.94 & 91.20 \\
 &$\epsilon$=0.05 & 54.86 & 71.99 & 84.03 & 91.20 \\
 &$\epsilon$=0.07 & 53.47 & 70.60 & 82.87 & 91.44 \\
 &$\epsilon$=0.09 & 54.86 & 71.53 & 77.31 & 88.43 \\
\midrule
\multirow{6}{2em}{i-fgsm}&baseline&na& 58.42 & 76.37 & 88.83 \\
 &$\epsilon$=0.01 & 46.00 & 63.24 & 77.21 & 90.14 \\
 &$\epsilon$=0.03 & 45.79 & 62.42 & 73.92 & 87.89 \\
 &$\epsilon$=0.05 & 43.74 & 64.27 & 75.77 & 89.32 \\
 &$\epsilon$=0.07 & 46.20 & 62.83 & 77.62 & 89.53 \\
 &$\epsilon$=0.09 & 43.33 & 63.45 & 71.46 & 84.39 \\

\bottomrule
\end{tabular}
\end{sc}
\end{small}
\end{center}
\vskip -0.1in
\begin{tablenotes}
      \small
      \item The five cells 
    \end{tablenotes}
  \end{threeparttable}
\end{table}

\begin{table}[t]
\begin{threeparttable}
\caption{Transformation ensemble performance in different neighborhood with VGG19 on Blackbox Attack 7 noise}
\label{sample-table}
\vskip 0.15in
\begin{center}
\begin{small}
\begin{sc}
\begin{tabular}{lccccr}
\toprule
attack&detection   &     2\% &    5\% &    10\% &    20\% \\
\midrule
\multirow{6}{2em}{AUG-PGD}&baseline& na&60.61 & 85.19  & 95.29 \\
&$\epsilon$=0.01 & 49.81 & 74.72 & 84.39 & 93.68 \\
 &$\epsilon$=0.03 & 49.63 & 72.22 & 80.74 & 92.22 \\
 &$\epsilon$=0.05 & 51.85 & 73.33 & 84.44 & 91.85 \\
 &$\epsilon$=0.07 & 52.59 & 72.22 & 82.59 & 91.11 \\
 &$\epsilon$=0.09 & 49.63 & 67.41 & 77.78 & 90.74 \\
\midrule
\multirow{6}{2em}{Alt-PGD}&baseline&na& 64.58 & 83.07 & 93.73 \\
 &$\epsilon$=0.01 & 54.77 & 75.62 & 83.39 & 93.64 \\
 &$\epsilon$=0.03 & 57.39 & 74.30 & 82.75 & 91.90 \\
 &$\epsilon$=0.05 & 58.10 & 75.35 & 87.32 & 92.61 \\
 &$\epsilon$=0.07 & 57.75 & 76.41 & 84.15 & 91.90 \\
 &$\epsilon$=0.09 & 54.93 & 73.24 & 80.28 & 90.49 \\
\midrule
\multirow{6}{2em}{fgsm}&baseline&na& 59.00 & 80.33  & 91.84 \\
&$\epsilon$=0.01 & 53.43 & 71.16 & 80.14 & 91.96 \\
 &$\epsilon$=0.03 & 52.36 & 68.63 & 78.54 & 91.04 \\
 &$\epsilon$=0.05 & 52.59 & 69.10 & 79.25 & 90.80 \\
 &$\epsilon$=0.07 & 51.18 & 69.81 & 78.07 & 90.57 \\
 &$\epsilon$=0.09 & 45.99 & 65.33 & 76.65 & 87.03 \\
\midrule
\multirow{6}{2em}{t-fgsm}&baseline&na& 59.71 & 83.47 & 95.04 \\
 &$\epsilon$=0.01 & 55.22 & 74.94 & 86.31 & 93.50 \\
 &$\epsilon$=0.03 & 54.86 & 72.92 & 81.94 & 92.36 \\
 &$\epsilon$=0.05 & 56.71 & 71.99 & 83.33 & 93.06 \\
 &$\epsilon$=0.07 & 56.48 & 73.84 & 81.71 & 92.36 \\
 &$\epsilon$=0.09 & 49.31 & 68.75 & 79.40 & 89.58 \\
\midrule
\multirow{6}{2em}{i-fgsm}&baseline&na& 58.42 & 76.37 & 88.83 \\
 &$\epsilon$=0.01 & 47.33 & 65.84 & 79.63 & 91.56 \\
 &$\epsilon$=0.03 & 47.64 & 63.66 & 75.77 & 90.35 \\
 &$\epsilon$=0.05 & 47.64 & 64.48 & 77.21 & 89.94 \\
 &$\epsilon$=0.07 & 46.82 & 65.09 & 76.39 & 89.53 \\
 &$\epsilon$=0.09 & 41.27 & 63.66 & 74.54 & 85.83 \\

\bottomrule
\end{tabular}
\end{sc}
\end{small}
\end{center}
\vskip -0.1in
\begin{tablenotes}
      \small
      \item The five cells 
    \end{tablenotes}
  \end{threeparttable}
\end{table}

\begin{table}[t]
\begin{threeparttable}
\caption{L1 distance performance in different neighborhood with VGG19 on Greybox Attack 1 noise}
\label{sample-table}
\vskip 0.15in
\begin{center}
\begin{small}
\begin{sc}
\begin{tabular}{lccccr}
\toprule
attack & detection   &     2\% &    5\% &    10\% &    20\% \\
\midrule
 \multirow{6}{2em}{AUG-PGD}&baseline &na& 82.38 & 88.99 & 94.39 \\
 &$\epsilon$=0.01 & 81.11 & 90.67 & 94.22 & 97.11 \\
 &$\epsilon$=0.03 & 79.22 & 90.00 & 94.67 & 96.89 \\
 &$\epsilon$=0.05 & 77.44 & 91.22 & 95.33 & 97.78 \\
 &$\epsilon$=0.07 & 71.44 & 90.89 & 96.56 & 98.56 \\
 &$\epsilon$=0.09 & 68.33 & 89.56 & 96.11 & 98.67 \\
\midrule
 \multirow{6}{2em}{Alt-PGD}&baseline &na& 72.14 & 77.96 & 87.88 \\
 &$\epsilon$=0.01 & 75.53 & 83.31 & 89.43 & 93.21 \\
 &$\epsilon$=0.03 & 78.42 & 84.32 & 88.32 & 93.99 \\
 &$\epsilon$=0.05 & 80.65 & 86.43 & 91.43 & 95.11 \\
 &$\epsilon$=0.07 & 80.87 & 88.43 & 92.77 & 96.77 \\
 &$\epsilon$=0.09 & 83.20 & 88.43 & 92.66 & 96.33 \\
 \midrule
 \multirow{6}{2em}{FGSM}&baseline &na& 38.20 & 57.54 & 74.57 \\
 &$\epsilon$=0.01 &  8.68 & 24.83 & 45.73 & 74.36 \\
 &$\epsilon$=0.03 &  8.41 & 21.17 & 42.06 & 70.83 \\
 &$\epsilon$=0.05 &  7.60 & 18.72 & 38.94 & 70.01 \\
 &$\epsilon$=0.07 &  6.65 & 15.74 & 36.64 & 70.01 \\
 &$\epsilon$=0.09 &  7.73 & 18.18 & 35.82 & 67.30 \\
 \midrule
 \multirow{6}{2em}{T-FGSM}&baseline &na& 40.85 & 63.00 & 81.56 \\
 &$\epsilon$=0.01 &  9.23 & 25.14 & 43.47 & 77.41 \\
 &$\epsilon$=0.03 &  7.24 & 19.03 & 39.49 & 73.86 \\
 &$\epsilon$=0.05 &  7.39 & 17.61 & 38.92 & 69.89 \\
 &$\epsilon$=0.07 &  6.68 & 16.76 & 35.37 & 65.91 \\
 &$\epsilon$=0.09 &  5.97 & 15.34 & 32.67 & 62.78 \\
 \midrule
 \multirow{6}{2em}{I-FGSM}&baseline &na& 41.49 & 51.89 & 65.55 \\
 &$\epsilon$=0.01 & 44.75 & 57.85 & 67.46 & 80.00 \\
 &$\epsilon$=0.03 & 46.21 & 56.72 & 67.57 & 80.79 \\
 &$\epsilon$=0.05 & 47.91 & 57.51 & 70.96 & 82.26 \\
 &$\epsilon$=0.07 & 47.12 & 57.97 & 71.07 & 83.39 \\
 &$\epsilon$=0.09 & 50.17 & 60.11 & 72.99 & 84.97 \\

\bottomrule
\end{tabular}
\end{sc}
\end{small}
\end{center}
\vskip -0.1in
\begin{tablenotes}
      \small
      \item The five cells 
    \end{tablenotes}
  \end{threeparttable}
\end{table}

\begin{table}[t]
\begin{threeparttable}
\caption{L1 distance performance in different neighborhood with VGG19 on Greybox Attack 3 noises}
\label{sample-table}
\vskip 0.15in
\begin{center}
\begin{small}
\begin{sc}
\begin{tabular}{lccccr}
\toprule
attack & detection   &     2\% &    5\% &    10\% &    20\% \\
\midrule
 \multirow{6}{2em}{AUG-PGD}&baseline &na& 82.38 & 88.99 & 94.39 \\
 &$\epsilon$=0.01 & 79.89 & 90.33 & 95.22 & 97.67 \\
 &$\epsilon$=0.03 & 71.78 & 89.22 & 93.56 & 97.33 \\
 &$\epsilon$=0.05 & 64.33 & 89.22 & 95.44 & 98.00 \\
 &$\epsilon$=0.07 & 56.00 & 84.67 & 95.11 & 98.56 \\
 &$\epsilon$=0.09 & 53.56 & 82.89 & 95.22 & 98.44 \\
\midrule
 \multirow{6}{2em}{Alt-PGD}&baseline &na& 72.14 & 77.96 & 87.88 \\
&$\epsilon$=0.01 & 77.75 & 84.87 & 89.21 & 93.77 \\
 &$\epsilon$=0.03 & 81.87 & 86.87 & 90.43 & 94.88 \\
 &$\epsilon$=0.05 & 82.87 & 90.32 & 93.21 & 96.44 \\
 &$\epsilon$=0.07 & 83.65 & 90.21 & 94.33 & 97.22 \\
 &$\epsilon$=0.09 & 85.54 & 91.32 & 94.44 & 96.66 \\
 \midrule
 \multirow{6}{2em}{FGSM}&baseline &na& 38.20 & 57.54 & 74.57 \\
 &$\epsilon$=0.01 &  8.01 & 21.98 & 40.57 & 71.23 \\
 &$\epsilon$=0.03 &  5.56 & 14.65 & 33.11 & 65.13 \\
 &$\epsilon$=0.05 &  4.75 & 14.65 & 27.95 & 63.23 \\
 &$\epsilon$=0.07 &  4.75 & 13.43 & 29.58 & 62.96 \\
 &$\epsilon$=0.09 &  6.11 & 14.11 & 30.26 & 56.58 \\
 \midrule
 \multirow{6}{2em}{T-FGSM}&baseline &na& 40.85 & 63.00 & 81.56 \\
 &$\epsilon$=0.01 &  8.95 & 21.16 & 40.34 & 74.01 \\
 &$\epsilon$=0.03 &  5.40 & 15.77 & 33.81 & 65.48 \\
 &$\epsilon$=0.05 &  3.41 & 13.49 & 29.12 & 59.52 \\
 &$\epsilon$=0.07 &  4.40 & 13.21 & 28.98 & 59.09 \\
 &$\epsilon$=0.09 &  4.12 & 11.08 & 25.00 & 52.70 \\
 \midrule
 \multirow{6}{2em}{I-FGSM}&baseline &na& 41.49 & 51.89 & 65.55 \\
 &$\epsilon$=0.01 & 47.34 & 58.87 & 68.47 & 79.66 \\
 &$\epsilon$=0.03 & 46.78 & 57.18 & 69.27 & 82.15 \\
 &$\epsilon$=0.05 & 46.78 & 59.89 & 69.38 & 83.16 \\
 &$\epsilon$=0.07 & 48.14 & 62.26 & 73.45 & 86.44 \\
 &$\epsilon$=0.09 & 52.99 & 66.33 & 76.72 & 88.81 \\

\bottomrule
\end{tabular}
\end{sc}
\end{small}
\end{center}
\vskip -0.1in
\begin{tablenotes}
      \small
      \item The five cells 
    \end{tablenotes}
  \end{threeparttable}
\end{table}

\begin{table}[t]
\begin{threeparttable}
\caption{L1 distance performance in different neighborhood with VGG19 on Greybox Attack 7 noises}
\label{sample-table}
\vskip 0.15in
\begin{center}
\begin{small}
\begin{sc}
\begin{tabular}{lccccr}
\toprule
attack & detection   &     2\% &    5\% &    10\% &    20\% \\
\midrule
 \multirow{6}{2em}{AUG-PGD}&baseline &na& 82.38 & 88.99 & 94.39 \\
 &$\epsilon$=0.01 & 75.78 & 90.22 & 94.22 & 97.33 \\
 &$\epsilon$=0.03 & 60.78 & 88.56 & 94.44 & 97.22 \\
 &$\epsilon$=0.05 & 55.67 & 85.78 & 95.44 & 98.33 \\
 &$\epsilon$=0.07 & 45.67 & 81.00 & 95.33 & 98.78 \\
 &$\epsilon$=0.09 & 39.00 & 76.00 & 93.78 & 98.78 \\
\midrule
 \multirow{6}{2em}{Alt-PGD}&baseline &na& 72.14 & 77.96 & 87.88 \\
&$\epsilon$=0.01 & 77.31 & 84.87 & 89.32 & 93.21 \\
 &$\epsilon$=0.03 & 80.53 & 88.10 & 91.77 & 95.11 \\
 &$\epsilon$=0.05 & 85.21 & 91.88 & 94.77 & 96.55 \\
 &$\epsilon$=0.07 & 85.32 & 92.88 & 94.99 & 97.55 \\
 &$\epsilon$=0.09 & 86.76 & 92.55 & 94.99 & 97.11 \\
 \midrule
 \multirow{6}{2em}{FGSM}&baseline &na& 38.20 & 57.54 & 74.57 \\
 &$\epsilon$=0.01 &  7.60 & 19.00 & 37.99 & 70.42 \\
 &$\epsilon$=0.03 &  3.80 & 13.30 & 29.44 & 63.91 \\
 &$\epsilon$=0.05 &  3.66 & 12.75 & 27.00 & 58.21 \\
 &$\epsilon$=0.07 &  5.29 & 12.89 & 26.87 & 55.22 \\
 &$\epsilon$=0.09 &  5.43 & 12.89 & 25.24 & 48.44 \\
 \midrule
 \multirow{6}{2em}{T-FGSM}&baseline &na& 40.85 & 63.00 & 81.56 \\
&$\epsilon$=0.01 &  7.10 & 17.61 & 37.93 & 71.59 \\
 &$\epsilon$=0.03 &  3.27 & 13.49 & 26.70 & 59.80 \\
 &$\epsilon$=0.05 &  3.27 & 10.09 & 24.43 & 56.39 \\
 &$\epsilon$=0.07 &  3.12 & 10.65 & 22.30 & 50.57 \\
 &$\epsilon$=0.09 &  3.84 &  9.66 & 20.17 & 43.32 \\
 \midrule
 \multirow{6}{2em}{I-FGSM}&baseline &na& 41.49 & 51.89 & 65.55 \\
&$\epsilon$=0.01 & 48.36 & 57.97 & 70.17 & 81.13 \\
 &$\epsilon$=0.03 & 45.31 & 59.55 & 70.62 & 82.49 \\
 &$\epsilon$=0.05 & 48.47 & 61.47 & 72.20 & 85.65 \\
 &$\epsilon$=0.07 & 50.06 & 66.10 & 76.72 & 88.59 \\
 &$\epsilon$=0.09 & 47.91 & 65.42 & 75.48 & 87.12 \\

\bottomrule
\end{tabular}
\end{sc}
\end{small}
\end{center}
\vskip -0.1in
\begin{tablenotes}
      \small
      \item The five cells 
    \end{tablenotes}
  \end{threeparttable}
\end{table}

\begin{table}[t]
\begin{threeparttable}
\caption{Transformation ensemble performance in different neighborhood with VGG19 on Blackbox Attack 1 noise}
\label{sample-table}
\vskip 0.15in
\begin{center}
\begin{small}
\begin{sc}
\begin{tabular}{lccccr}
\toprule
attack&detection   &     2\% &    5\% &    10\% &    20\% \\
\midrule
\multirow{6}{2em}{AUG-PGD}&baseline& na&60.61 & 85.19  & 95.29 \\
&$\epsilon$=0.01 &  5.93 & 20.37 & 42.22 & 81.85 \\
 &$\epsilon$=0.03 &  2.96 & 11.85 & 31.48 & 68.52 \\
 &$\epsilon$=0.05 &  2.22 & 11.11 & 30.74 & 68.89 \\
 &$\epsilon$=0.07 &  2.59 &  7.04 & 22.96 & 62.96 \\
 &$\epsilon$=0.09 &  1.85 &  7.41 & 17.41 & 57.41 \\
\midrule
\multirow{6}{2em}{Alt-PGD}&baseline&na& 64.58 & 83.07 & 93.73 \\
&$\epsilon$=0.01 &  9.51 & 21.83 & 42.96 & 82.39 \\
 &$\epsilon$=0.03 &  7.39 & 17.96 & 36.62 & 72.54 \\
 &$\epsilon$=0.05 &  8.45 & 14.44 & 33.80 & 69.37 \\
 &$\epsilon$=0.07 &  6.34 & 13.38 & 28.52 & 61.62 \\
 &$\epsilon$=0.09 &  5.99 & 13.38 & 24.65 & 60.21 \\
\midrule
\multirow{6}{2em}{fgsm}&baseline&na& 59.00 & 80.33  & 91.84 \\
&$\epsilon$=0.01 &  8.49 & 23.11 & 48.11 & 82.55 \\
 &$\epsilon$=0.03 &  7.55 & 17.69 & 39.86 & 78.07 \\
 &$\epsilon$=0.05 &  5.90 & 13.92 & 36.08 & 72.88 \\
 &$\epsilon$=0.07 &  6.13 & 12.03 & 29.01 & 67.69 \\
 &$\epsilon$=0.09 &  4.01 & 10.61 & 25.71 & 60.38 \\
\midrule
\multirow{6}{2em}{t-fgsm}&baseline&na& 59.71 & 83.47 & 95.04 \\
 &$\epsilon$=0.01 &  8.80 & 23.38 & 46.30 & 83.10 \\
 &$\epsilon$=0.03 &  7.87 & 19.91 & 38.66 & 76.39 \\
 &$\epsilon$=0.05 &  4.86 & 14.81 & 32.18 & 69.68 \\
 &$\epsilon$=0.07 &  3.01 & 12.96 & 26.16 & 63.89 \\
 &$\epsilon$=0.09 &  3.47 & 10.42 & 23.38 & 57.18 \\
\midrule
\multirow{6}{2em}{i-fgsm}&baseline&na& 58.42 & 76.37 & 88.83 \\
 &$\epsilon$=0.01 & 22.59 & 41.48 & 58.93 & 85.01 \\
 &$\epsilon$=0.03 & 17.66 & 32.65 & 51.13 & 77.62 \\
 &$\epsilon$=0.05 & 18.69 & 29.16 & 48.05 & 75.36 \\
 &$\epsilon$=0.07 & 15.40 & 26.69 & 46.00 & 74.54 \\
 &$\epsilon$=0.09 & 12.94 & 25.67 & 42.71 & 70.43 \\

\bottomrule
\end{tabular}
\end{sc}
\end{small}
\end{center}
\vskip -0.1in
\begin{tablenotes}
      \small
      \item The five cells 
    \end{tablenotes}
  \end{threeparttable}
\end{table}

\begin{table}[t]
\begin{threeparttable}
\caption{Transformation ensemble performance in different neighborhood with VGG19 on Blackbox Attack 7 noises}
\label{sample-table}
\vskip 0.15in
\begin{center}
\begin{small}
\begin{sc}
\begin{tabular}{lccccr}
\toprule
attack&detection   &     2\% &    5\% &    10\% &    20\% \\
\midrule
\multirow{6}{2em}{AUG-PGD}&baseline& na&60.61 & 85.19  & 95.29 \\
 &$\epsilon$=0.01 &  2.59 & 10.74 & 30.00 & 65.93 \\
 &$\epsilon$=0.03 &  1.85 &  5.19 & 17.04 & 52.22 \\
 &$\epsilon$=0.05 &  0.37 &  2.22 & 11.11 & 40.00 \\
 &$\epsilon$=0.07 &  1.11 &  3.33 &  9.26 & 33.70 \\
 &$\epsilon$=0.09 &  0.00 &  0.37 &  0.37 &  1.48 \\
\midrule
\multirow{6}{2em}{Alt-PGD}&baseline&na& 64.58 & 83.07 & 93.73 \\
&$\epsilon$=0.01 &  8.45 & 15.85 & 34.86 & 68.31 \\
 &$\epsilon$=0.03 &  6.69 & 12.32 & 22.18 & 50.70 \\
 &$\epsilon$=0.05 &  3.52 &  9.86 & 20.77 & 44.37 \\
 &$\epsilon$=0.07 &  1.76 &  8.45 & 16.20 & 39.79 \\
 &$\epsilon$=0.09 &  0.00 &  0.00 &  1.06 &  2.46 \\
\midrule
\multirow{6}{2em}{fgsm}&baseline&na& 59.00 & 80.33  & 91.84 \\
&$\epsilon$=0.01 &  7.78 & 15.33 & 38.21 & 73.11 \\
 &$\epsilon$=0.03 &  4.95 & 11.32 & 22.41 & 59.91 \\
 &$\epsilon$=0.05 &  4.01 &  9.67 & 18.63 & 47.64 \\
 &$\epsilon$=0.07 &  2.59 &  7.08 & 15.57 & 40.80 \\
 &$\epsilon$=0.09 &  0.00 &  0.00 &  0.47 &  2.83 \\
\midrule
\multirow{6}{2em}{t-fgsm}&baseline&na& 59.71 & 83.47 & 95.04 \\
 &$\epsilon$=0.01 &  6.02 & 16.67 & 37.27 & 71.53 \\
 &$\epsilon$=0.03 &  2.78 & 10.42 & 27.31 & 56.02 \\
 &$\epsilon$=0.05 &  2.08 &  6.94 & 19.44 & 45.37 \\
 &$\epsilon$=0.07 &  1.62 &  6.02 & 15.05 & 38.89 \\
 &$\epsilon$=0.09 &  0.00 &  0.23 &  0.46 &  1.39 \\
\midrule
\multirow{6}{2em}{i-fgsm}&baseline&na& 58.42 & 76.37 & 88.83 \\
 &$\epsilon$=0.01 & 19.10 & 32.65 & 51.54 & 78.03 \\
 &$\epsilon$=0.03 & 12.53 & 24.85 & 41.27 & 68.17 \\
 &$\epsilon$=0.05 &  9.24 & 22.18 & 33.88 & 59.55 \\
 &$\epsilon$=0.07 &  7.80 & 18.89 & 31.83 & 57.70 \\
 &$\epsilon$=0.09 &  0.41 &  1.03 &  3.29 &  8.62 \\

\bottomrule
\end{tabular}
\end{sc}
\end{small}
\end{center}
\vskip -0.1in
\begin{tablenotes}
      \small
      \item The five cells 
    \end{tablenotes}
  \end{threeparttable}
\end{table}
}
